# Supplementary material for: Testing Theories of Gravity with Planetary Ephemerides
Source: arXiv:2303.01821 source file (2023-07-25)
Supplement: Supplementary file 1 [file appendice_EP+SH.tex]

\section{Impact on EP for the Shapiro correction}

It has been explained in Sect \ref{xx} that for the computation of the Shapiro delay one has to account for m$_I$ instead of m$_g$. The effect is lower than the millimeter level as one can see on Fig. \ref{fig:BCMImBCMG}.

\begin{figure}
    \centering
    \includegraphics[scale=0.5]{Figures/BCMImBCMG}
    \caption{Differences for simulated Bepi-Colombo Earth-Mercury distances between Shapiro delay estimated with  m$_I$ and with  m$_g$ in millimeter  }
    \label{fig:BCMImBCMG}
\end{figure}

If one consider the relative differences, in some configurations, the ratio between the differences in residuals and the residuals can reach 300$\%$ before fit.

\begin{figure}
    \centering
    \includegraphics[scale=0.3]{Figures/relative}
    \caption{Top: Dilaton residuals for $\alpha_0=10^{-4}$ before fit in meters. Middle: Differences for simulated Bepi-Colombo Earth-Mercury distances between Shapiro delay estimated with  m$_I$ and with  m$_g$ in meters. Buttom: Ratio between the differences and the residuals  }
    \label{fig:relative}
\end{figure}
